# Supplementary material for: Suppression of errors in collectively coded information
Source: arXiv:2508.21806 source file (2025-09-24)

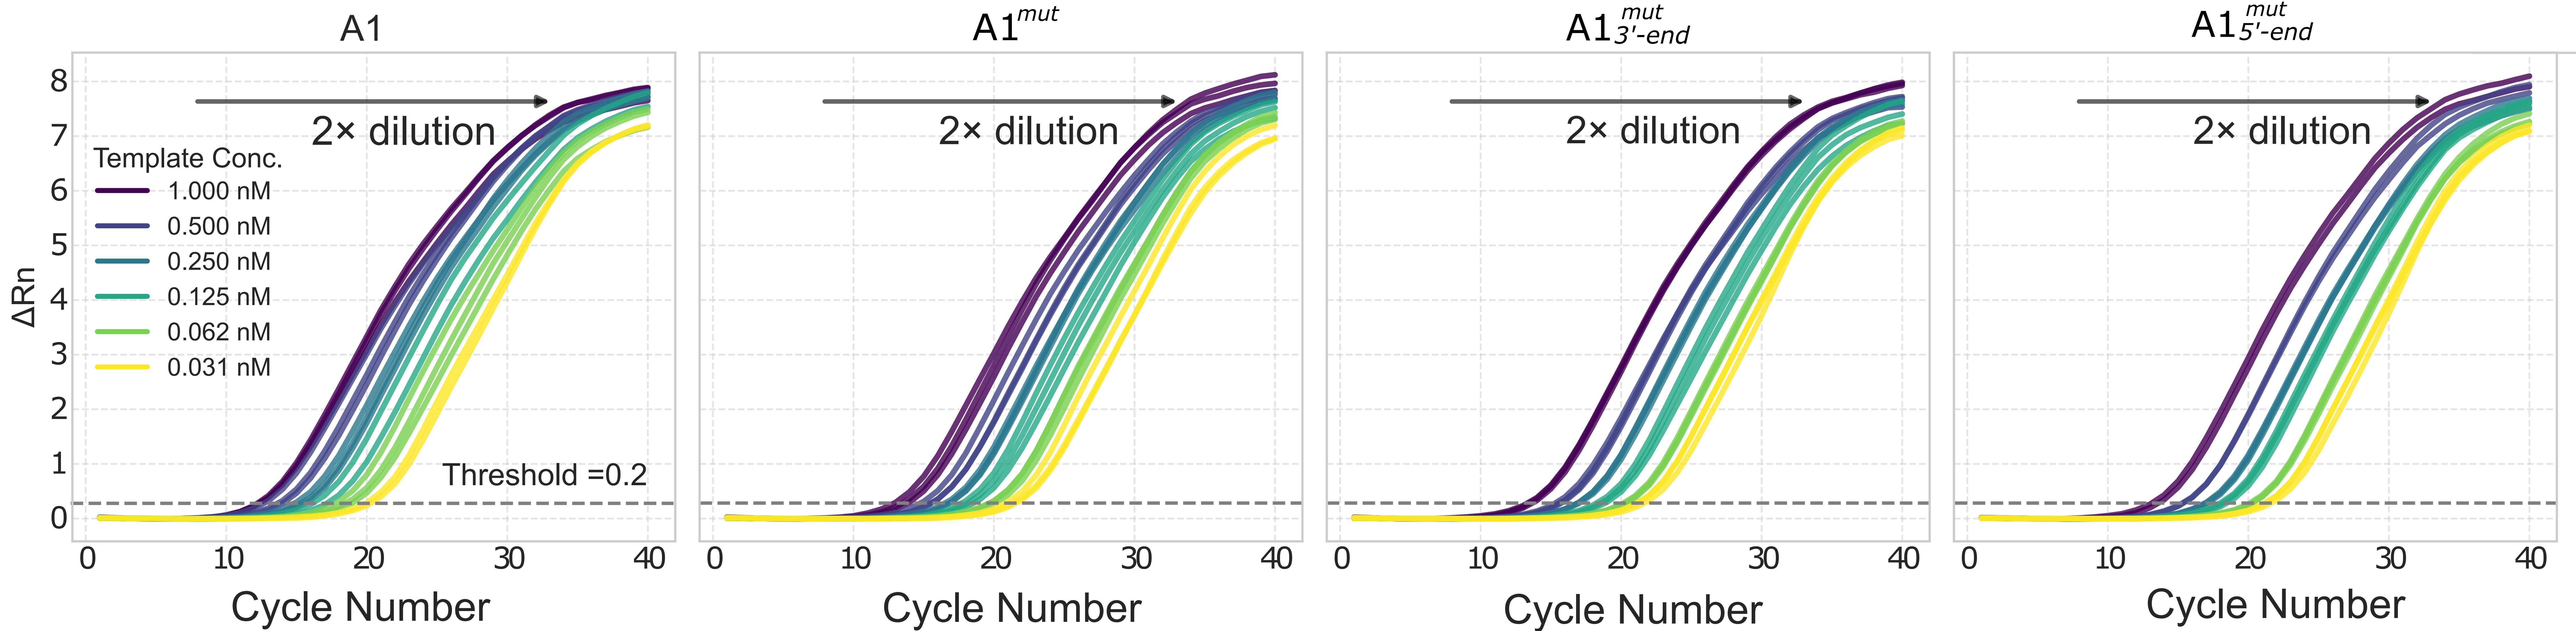

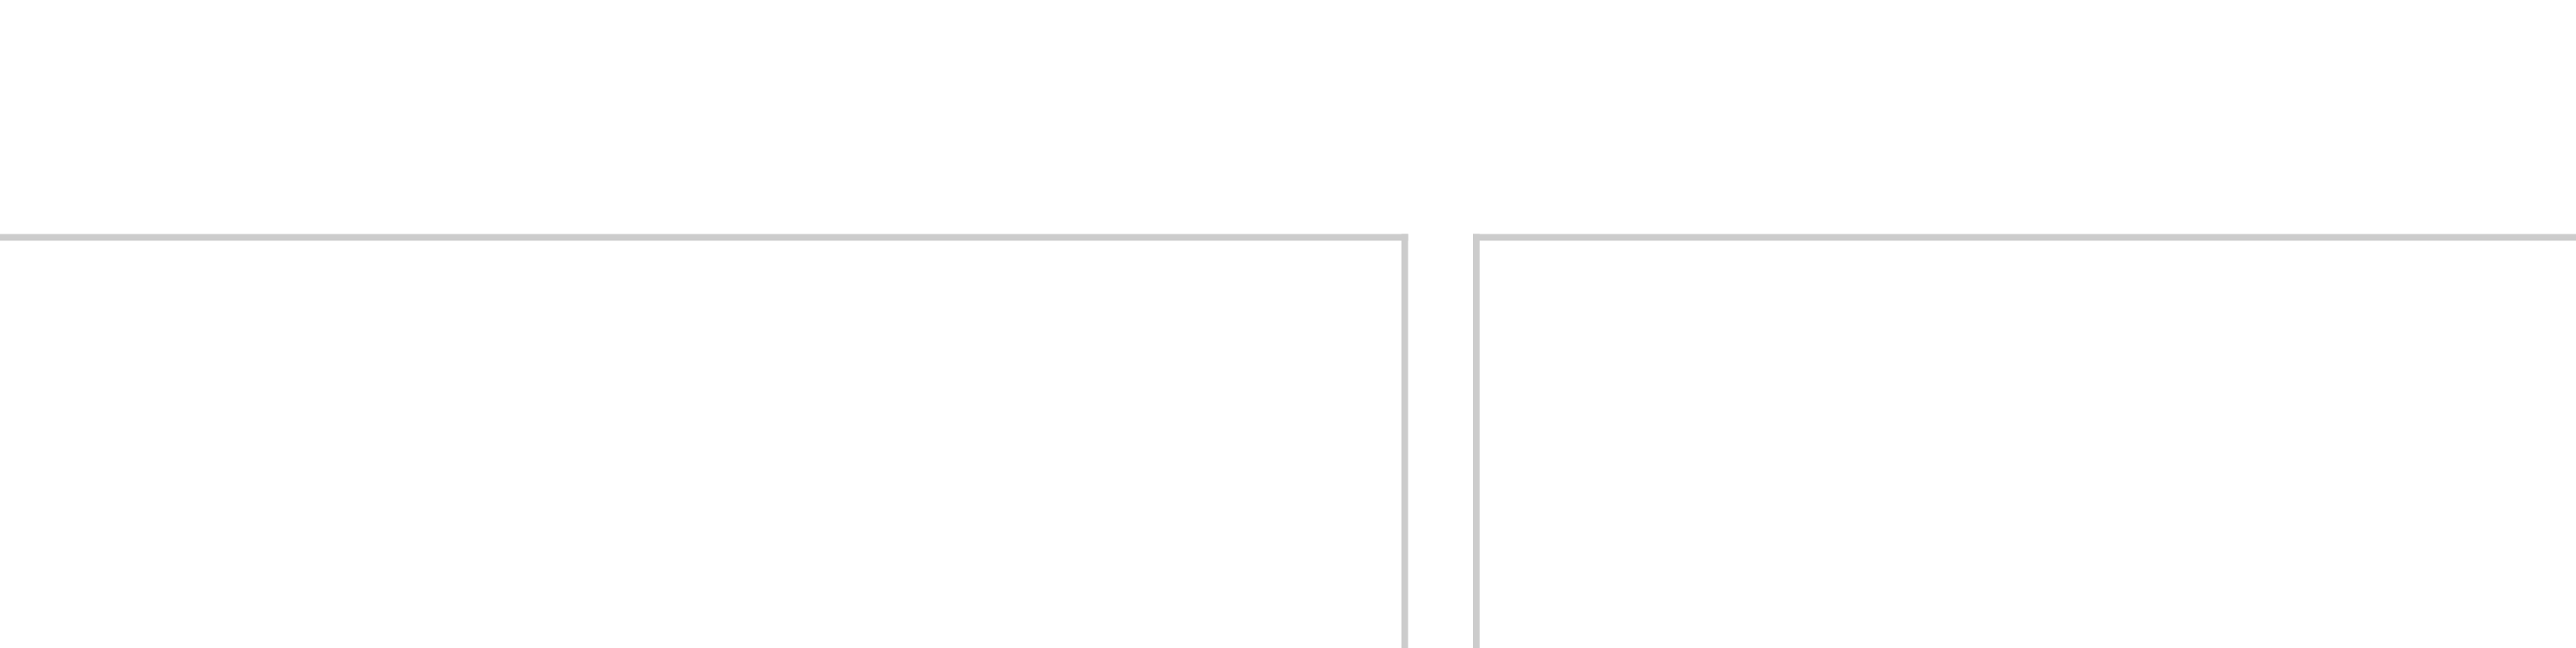

Supplement: Supplementary file 1 [file 20250620AmpCurve_control_cycle0_all_with_threshold.pdf]
